# Supplementary material for: Lazily Adapted Constant Kinky Inference for Nonparametric Regression and Model-Reference Adaptive Control
Source: arXiv:1701.00178 source file (2021-03-10)
Supplement: Supplementary file 1 [file KI_appendix.tex]

\chapter{Derivations and supplementary results pertaining to Ch. \ref{{ch:kinkyinf}}}
